# Supplementary material for: VULSOLVER: Vulnerability Detection via LLM-Driven Constraint Solving
Source: arXiv:2509.00882 source file (2025-11-25)
Supplement: Supplementary file 1 [file appendix.tex]

% \section{appendix}

% In this section, we will use a code audit example of a path traversal vulnerability to detail how VulDetector performs a human-like code audit.

% \subsection{Demo Source Code}
% DemoServlet.java

% \begin{verbatim}
% Omitted, no translation needed
% \end{verbatim}

% AnotherClass.java

% \begin{verbatim}
% Omitted, no translation needed
% \end{verbatim}

% SafeUtil.java

% \begin{verbatim}
% Omitted, no translation needed
% \end{verbatim}

% \subsection{Code Information Summary}
% With the help of SAST, the potential vulnerability call chain for path traversal is first identified:  
% \texttt{DemoServlet\#doGet -> DemoServlet\#node1 -> DemoServlet\#node2 -> DemoServlet\#node3 -> Files\#readAllBytes}

% Additional metadata for the potential vulnerability call chain is supplemented, generating the corresponding code information summary:

% \begin{itemize}
% \item Code details of methods on the vulnerability call chain and their branches:
%   \begin{itemize}
%   \item Class to which the method belongs
%   \item Method name
%   \item Method source code
%   \item Method parameter types and names
%   \end{itemize}
% \item Call information between methods on the vulnerability call chain and their branches:
%   \begin{itemize}
%   \item Call relationships between methods
%   \item The callee's expression in the caller's source code
%   \end{itemize}
% \item Type details:
%   \begin{itemize}
%   \item Class name
%   \item Member variable types and names
%   \item Whether it is a static type
%   \end{itemize}
% \item Data flow analysis information:
%   \begin{itemize}
%   \item Data flow relationships between methods
%   \item Data flow relationships within methods
%   \end{itemize}
% \end{itemize}

% \subsection{Key Types, Non-Exploitable Conditions, and Vulnerability Exploitability Determination}
% VulDetector defines different key types and non-exploitable conditions for different vulnerability types. The exploitability of all sink methods is determined by the logical combination of key types and non-exploitable conditions within the sink methods.

% \subsubsection{Key Types and Non-Exploitable Conditions}
% Taking this demo as an example, the key types and non-exploitable conditions for path traversal vulnerabilities are:

% \begin{itemize}
% \item File: 'the file path of key variable will not contain ".."'  
% \item Path: 'the file path of key variable will not contain ".."'  
% \item URI: 'the file path of key variable will not contain ".."'  
% \item FileDescriptor: 'the file path of key variable will not contain ".."'  
% \item String: 'key variable will not contain ".."'  
% \item RandomAccessFile: 'the file path of key variable will not contain ".."'  
% \item FileOutputStream: 'the file path of key variable will not contain ".."'  
% \item OutputStream: 'key variable is not a file output stream or the file path of key variable will not contain ".."'
% \end{itemize}

% \subsubsection{Vulnerability Exploitability Determination}
% The condition for determining whether the sink method \texttt{Files\#readAllBytes} can be exploited is: When the method \texttt{public static byte[] readAllBytes(Path path)} is executed through the above call chain, does its key type parameter \texttt{Path path} necessarily satisfy \texttt{the file path of key_variable will not contain ".."}?

% \subsection{Constraint Solving Process}
% The following sections will sequentially outline the entire constraint-solving process.

% \subsubsection{DemoServlet\#doGet -> DemoServlet\#node1}
% \paragraph{Analysis Goal:}
% In the definition of \texttt{DemoServlet\#node1}, \texttt{public String node1(String param1, String param2)}, both \texttt{param1} and \texttt{param2} are key types. Therefore, the analysis goals are:

% \begin{itemize}
% \item Goal 1: When \texttt{DemoServlet\#node1} is called in \texttt{DemoServlet\#doGet}, does \texttt{param1} satisfy \texttt{'param1 will not contain ".."'}?
% \item Goal 2: When \texttt{DemoServlet\#node1} is called in \texttt{DemoServlet\#doGet}, does \texttt{param2} satisfy \texttt{'param2 will not contain ".."'}?
% \end{itemize}

% Here, Goal 1 is used as an example:

% \paragraph{Context:}
% As the entry point for web requests, no additional context is needed.

% The called branch methods are well-known and do not require separate analysis.

% \paragraph{Prompt Construction}
% Given:

% \begin{itemize}
% \item \texttt{DemoServlet\#doGet} calls \texttt{DemoServlet\#node1}
% \item The code for \texttt{DemoServlet\#doGet} is provided
% \end{itemize}

% Solve:

% \begin{itemize}
% \item When \texttt{DemoServlet\#node1} is called, does \texttt{param1} satisfy \texttt{'param1 will not contain ".."'}?
% \end{itemize}

% \paragraph{Expected Result}
% Since the code does not perform any filtering and directly passes the HTTP request parameters to \texttt{param1} and \texttt{param2}, the conclusion should be that the conditions are not satisfied.

% \subsubsection{DemoServlet\#node1 -> DemoServlet\#node2}
% \paragraph{Analysis Goal:}
% In the definition of \texttt{DemoServlet\#node2}, \texttt{public String node2(AnotherClass param1)}, \texttt{param1} is of type \texttt{AnotherClass}, which encapsulates the key type \texttt{String}. Therefore, the analysis goals are:

% \begin{itemize}
% \item Goal 1: When \texttt{DemoServlet\#node2} is called in \texttt{DemoServlet\#node1}, does \texttt{param1.member1} satisfy \texttt{'will not contain ".."'}?
% \item ...
% \item Goal 6: When \texttt{DemoServlet\#node2} is called in \texttt{DemoServlet\#node1}, does \texttt{param1.member6} satisfy \texttt{'will not contain ".."'}?
% \end{itemize}

% However, it can be determined in advance that in the subsequent main call chain \texttt{DemoServlet\#node2 -> DemoServlet\#node3 -> Files\#readAllBytes} and related branch code, \texttt{member3} to \texttt{member6} do not appear. Therefore, these member variables do not need to be analyzed, and the analysis goals are simplified to:

% \begin{itemize}
% \item Goal 1: When \texttt{DemoServlet\#node2} is called in \texttt{DemoServlet\#node1}, does \texttt{param1.member1} satisfy \texttt{'will not contain ".."'}?
% \item Goal 2: When \texttt{DemoServlet\#node2} is called in \texttt{DemoServlet\#node1}, does \texttt{param1.member2} satisfy \texttt{'will not contain ".."'}?
% \end{itemize}

% Here, Goal 1 is used as an example:

% \paragraph{Context:}
% Based on the results of the previous main chain analysis, when \texttt{DemoServlet\#node1} starts executing, the parameters \texttt{param1} and \texttt{param2} cannot guarantee \texttt{'will not contain ".."'}.

% In addition, the branch methods \texttt{AnotherClass\#setMember1} and \texttt{AnotherClass\#setMember2} called here require semantic extraction via the branch analysis module. Here, \texttt{AnotherClass\#setMember1} is used as an example:

% \subparagraph{Branch: Analysis Goal}
% The parameter of \texttt{AnotherClass\#setMember1} is the key type \texttt{String}. Based on the method's parameter and return type, the semantic (analysis goal) to be extracted for this branch method is:

% The direction of data flow within \texttt{AnotherClass\#setMember1} (SAST reveals it flows from \texttt{param1} to \texttt{this.member1}), and whether the flow process results in the condition \texttt{'will not contain ".."'} being satisfied.

% \subparagraph{Branch: Prompt Construction}
% Given:

% \begin{itemize}
% \item The code for \texttt{AnotherClass\#setMember1} (since no additional methods are called, the call tree pruning result is only this method)
% \end{itemize}

% Solve:

% \begin{itemize}
% \item Does \texttt{this.member1} satisfy the non-exploitable condition?
% \end{itemize}

% \subparagraph{Branch: Expected Result}
% It can be seen that the code performs Base64 processing on the parameter, so the conclusion here should be that \texttt{this.member1} satisfies the non-exploitable condition.

% Similarly, the analysis conclusion for \texttt{AnotherClass\#setMember2} is that \texttt{this.member2} does not satisfy the non-exploitable condition.

% \paragraph{Prompt Construction}
% Given:

% \begin{itemize}
% \item \texttt{DemoServlet\#node1} calls \texttt{DemoServlet\#node2}
% \item The code for \texttt{DemoServlet\#node1} is provided
% \item When \texttt{DemoServlet\#node1} starts executing, the parameters \texttt{param1} and \texttt{param2} cannot guarantee \texttt{'will not contain ".."'}
% \item The branch method \texttt{AnotherClass\#setMember1} is semantically simplified as: Assigns \texttt{anotherClass.member1} a strictly filtered value that cannot contain \texttt{".."}
% \item The branch method \texttt{AnotherClass\#setMember2} is semantically simplified as: Assigns \texttt{param2} (the actual parameter of \texttt{AnotherClass\#setMember2}) to \texttt{anotherClass.member2}
% \end{itemize}

% Solve:

% \begin{itemize}
% \item Does \texttt{anotherClass.member1} satisfy the non-exploitable condition?
% \end{itemize}

% \paragraph{Expected Result}
% The LLM can observe that \texttt{anotherClass.member1} is assigned by \texttt{AnotherClass\#setMember1}, and the context indicates that this method assigns \texttt{anotherClass.member1} a strictly filtered value that cannot contain \texttt{".."}. Therefore, the LLM can conclude: \texttt{anotherClass.member1} satisfies the non-exploitable condition.

% Similarly, the LLM can determine that \texttt{anotherClass.member2} does not satisfy the non-exploitable condition.

% \subsubsection{DemoServlet\#node2 -> DemoServlet\#node3}
% \paragraph{Analysis Goal}
% In the definition of \texttt{DemoServlet\#node3}, \texttt{public String node3(String param1)}, \texttt{param1} is a key type. Therefore, the analysis goal is:

% \begin{itemize}
% \item Goal 1: When \texttt{DemoServlet\#node3} is called in \texttt{DemoServlet\#node2}, does \texttt{param1} satisfy \texttt{'will not contain ".."'}?
% \end{itemize}

% \paragraph{Context}
% Based on the results of the previous main chain analysis, when \texttt{DemoServlet\#node2} starts executing, \texttt{param1.member1} (converted from the actual parameter to the formal parameter in the previous analysis result) satisfies the non-exploitable condition, while \texttt{param1.member2} does not.

% In addition, the branch methods \texttt{SafeUtil\#filter} and \texttt{AnotherClass\#setMember2} called here require semantic extraction via the branch analysis module. \texttt{AnotherClass\#setMember2} has been explained earlier, and \texttt{param1.getPath()} is similar, so they are not repeated here. The handling of \texttt{SafeUtil\#filter} is described below:

% \subparagraph{Branch: Analysis Goal}
% The parameter of \texttt{SafeUtil\#filter} is the key type \texttt{String}, and the return type is \texttt{String}. Based on the method's parameter and return type, the semantic (analysis goal) to be extracted for this branch method is:

% The direction of data flow within \texttt{SafeUtil\#filter} (SAST reveals it flows from \texttt{param1} to \texttt{return}), and whether the flow process results in the condition \texttt{'will not contain ".."'} being satisfied.

% \subparagraph{Branch: Prompt Construction}
% Given:

% \begin{itemize}
% \item The code for \texttt{SafeUtil\#filter} (the other methods called are well-known, so the call tree pruning result is only this method)
% \end{itemize}

% Solve:

% \begin{itemize}
% \item Does \texttt{return} satisfy the non-exploitable condition?
% \end{itemize}

% \subparagraph{Branch: Expected Result}
% Very intuitively, \texttt{return} satisfies the non-exploitable condition.

% \paragraph{Prompt Construction}
% Given:

% \begin{itemize}
% \item \texttt{DemoServlet\#node2} calls \texttt{DemoServlet\#node3}
% \item The code for \texttt{DemoServlet\#node2} is provided
% \item When \texttt{DemoServlet\#node2} starts executing, \texttt{param1.member1} satisfies the non-exploitable condition, while \texttt{param1.member2} does not
% \item The branch method \texttt{SafeUtil\#filter} is semantically simplified as: Returns a strictly filtered value that cannot contain \texttt{".."}
% \item The branch method \texttt{AnotherClass\#setMember2} is semantically simplified as: Assigns \texttt{temp} (the actual parameter of \texttt{AnotherClass\#setMember2}) to \texttt{param1.member2}
% \item The branch method \texttt{param1.getPath()} is semantically simplified as: Returns \texttt{param1.member1 + param1.member2}
% \end{itemize}

% Solve:

% \begin{itemize}
% \item When \texttt{DemoServlet\#node3} is called, does \texttt{param1} satisfy the non-exploitable condition?
% \end{itemize}

% \paragraph{Expected Result}
% When \texttt{DemoServlet\#node3} is called, \texttt{param1} satisfies the non-exploitable condition.

% \subsubsection{DemoServlet\#node3 -> Files\#readAllBytes}
% \paragraph{Analysis Goal}
% In the definition of \texttt{Files\#readAllBytes}, \texttt{public static byte[] readAllBytes(Path path)}, \texttt{path} is a key type. Therefore, the analysis goal is:

% \begin{itemize}
% \item Goal 1: When \texttt{Files\#readAllBytes} is called in \texttt{DemoServlet\#node3}, does \texttt{path} satisfy \texttt{'the file path of path will not contain ".."'}?
% \end{itemize}

% \paragraph{Context}
% Based on the results of the previous main chain analysis, when \texttt{Files\#readAllBytes} starts executing, the parameter \texttt{param1} satisfies the non-exploitable condition.

% The called branch methods are well-known and do not require separate analysis.

% \paragraph{Prompt Construction}
% Given:

% \begin{itemize}
% \item \texttt{DemoServlet\#node3} calls \texttt{Files\#readAllBytes}
% \item The code for \texttt{DemoServlet\#node3} is provided
% \item When \texttt{DemoServlet\#node3} starts executing, the parameter \texttt{param1} satisfies the non-exploitable condition
% \end{itemize}

% Solve:

% \begin{itemize}
% \item When \texttt{Files\#readAllBytes} is called, does \texttt{path} satisfy the non-exploitable condition?
% \end{itemize}

% \paragraph{Expected Result}
% \begin{itemize}
% \item When \texttt{Files\#readAllBytes} is called, \texttt{path} satisfies the non-exploitable condition.
% \end{itemize}

% \subsection{Final Result}
% The final result of the analysis is that, under this call chain, when \texttt{Files\#readAllBytes} is executed:

% \texttt{'the file path of path will not contain ".."'}

% Therefore, no path traversal vulnerability exists here.

% This example is too complicated now, we need to find a more intuitive and simple example as an appendix. （https://www.yuque.com/g/lesion-jsgau/rk2xxd/uca36cvrwgsxy69c/collaborator/join?token=thc1lYYiGpyLm7Ov&source=doc_collaborator）
